# Supplementary material for: On the Core of the $b$-Matching Game
Source: arXiv:2502.01914 source file (2025-02-04)
Supplement: Supplementary file 1 [file appendix.tex]

% This file is for appendix section

\section{Appendix}
